# Supplementary material for: Expert Graphs: Synthesizing New Expertise via Collaboration
Source: arXiv:2107.07054 source file (2021-07-15)
Supplement: Supplementary file 1 [file One_vs_K.tex]

\subsection{Extending the Curl Condition to Multi-classifiers}
\label{apx:onevsk}
In previous sections, we considered pairwise experts, i.e. $1$ vs $1$ classifiers. In this section, we consider $1$ vs $k-1$ classifiers, where $k\geq 3$.
Given $\C$ such that $|\C|\geq k$, we define
\begin{align*}
  \hat{f}_x(C_{i_0},\cdots,C_{i_{k-1}})) &= \Pr(y = C_{i_0} \given y \in \{C_{i_0},\cdots, C_{i_{k-1}}\}, x)\\
    &= \frac{p_x^{(i_1)}}{\sum_{j=0}^{k-1}p_x^{(i_j)}}
\end{align*}
Given $k\geq 3$, $\C$, $\A$, $\ell \geq k$, $\curl_x(\C,\A,k)$ is defined as
\begin{equation}
    \curl_x(\C,\A,k) = \sum_{i=0}^{\ell-1}\hat{f}_x(C_{a_i},(C_{a_{i+1}},\cdots,C_{a_{i+k-1}}))
\end{equation}
For a distribution $d(\X)$, $\curl_d(\C,\A,k)$ is defined as 
\begin{equation}\label{eq:curl_d_general_k}
    \curl_d(\C,\A,k) = \E_d[
    \curl_x(\C,\A,k)]
\end{equation}
\begin{lem}\label{lem:curl_d_general_k}
Given $x\in\X,\C,\A,k\geq 3$ and $\ell\geq k$, 
\begin{itemize}
\item $\ell = k:\quad\quad\quad \curl_x(\C,\A,k) = 1.$
\item $\ell > k:\quad\quad 1< \curl_x(\C,\A,k) < \ell-k+1.$
\end{itemize}
\end{lem}
\begin{IEEEproof}
For convenience, let $p_x^{(a_0)},p_x^{(a_1)},\cdots,p_x^{(a_{\ell-1})}$ be denoted by a sequence $R = r_0, r_1, \cdots, r_{\ell-1}$ such that $r_i = p_x^{(a_i)}~\forall~i\in[\ell]$, define \[S_R(\ell,k) = \curl_x(\C,\A,k) =  \sum_{i=0}^{\ell-1}\frac{r_i}{\sum_{j=i}^{i+k-1}r_j}\]
We will prove the statement of the theorem using induction on $\ell$.
\begin{itemize}
    \item Base case ($\ell = k$):  $S_R(k,k)$ is given by  
    \begin{align*}
        \sum_{i=0}^{k-1}\frac{r_i}{\sum_{j=i}^{i+k-1}r_j}
        = \frac{\sum_{j=0}^{k-1}r_j}{\sum_{j=0}^{k-1}r_j} 
        = 1.
    \end{align*}
    \item Induction assumption
    \begin{itemize}
        \item \emph{Upper bound:} $$S_R(\ell,k) < \ell-k+1 \quad \forall R, k<\ell\leq L.$$
        \item \emph{Lower bound:} $$S_R(\ell,k) > 1 \quad \forall R, k<\ell\leq L.$$
    \end{itemize} 
    
    \item To prove: 
    \begin{itemize}
        \item \emph{Upper bound:}$$S_R(L+1,k) < L-k.$$
        \item \emph{Lower bound:} $$S_R(L+1,k) > 1.$$
    \end{itemize}
    \begin{enumerate}
    \item \emph{Upper Bound:} Let $r_m = max_{i=0}^{L}{r_i}$. Consider $U = u_0,u_1,\cdots,u_L$ such that $u_i = r_{i+m}$, i.e. $U$ is a cyclic shift of $R$ by $m$. Then, it is trivial to observe that
    $$S_U(L+1,k) = S_R(L+1,k).$$
    \begin{align*}
        S_U(L+1,k) = \frac{u_0}{u_0+\sum_{j=1}^{k-1}u_j}+\sum_{i=1}^{L}\frac{u_i}{\sum_{j=i}^{i+k-1}u_j}\\
        \stackrel{(a)}< 1+\sum_{i=1}^{L}\frac{u_i}{\sum_{j=i}^{i+k-1}u_j}\\
        = 1+\sum_{i=1}^{L-k+1}\frac{u_i}{\sum_{j=i}^{i+k-1}u_j}+\sum_{i=L-k+2}^{L}\frac{u_i}{u_0+\sum_{\substack{j=i\\ j\neq 0}}^{i+k-1}u_j}\\
        \stackrel{(b)}\leq 1+\sum_{i=1}^{L-k+1}\frac{u_i}{\sum_{j=i}^{i+k-1}u_j}+\sum_{i=L-k+2}^{L}\frac{u_i}{u_{i+k}+\sum_{\substack{j=i\\ j\neq 0}}^{i+k-1}u_j}\\
        \stackrel{(c)}= 1+S_{U'}(L,k)\\
        \stackrel{(d)}< 1+L-k-1\\
        =L-k.
    \end{align*}
    Here $(a)$ follows from $\frac{u_0}{u_0+\sum_{j=1}^{k-1}u_j}< 1$, $(b)$ follows from $u_0 = max_{i=0}^{L}{u_i}$, $(c)$ follows by assuming $U' = u_1,u_2,\cdots, u_L$ and $(d)$ follows from the induction assumption for the upper bound.  
\item \emph{Lower Bound:} Let $r_t = min_{i=0}^{L}{r_i}$. Consider $V = v_0,v_1,\cdots,v_L$ such that $v_i = r_{i+t}$, i.e. $V$ is a cyclic shift of $R$ by $t$. Then, it is trivial to observe that
    $$S_V(L+1,k) = S_R(L+1,k).$$
    \begin{align*}
        S_V(L+1,k) = \frac{v_0}{v_0+\sum_{j=1}^{k-1}v_j}+\sum_{i=1}^{L}\frac{v_i}{\sum_{j=i}^{i+k-1}v_j}\\
        \stackrel{(a)}> \sum_{i=1}^{L}\frac{v_i}{\sum_{j=i}^{i+k-1}v_j}\\
        = \sum_{i=1}^{L-k+1}\frac{v_i}{\sum_{j=i}^{i+k-1}v_j}+\sum_{i=L-k+2}^{L}\frac{v_i}{v_0+\sum_{\substack{j=i\\ j\neq 0}}^{i+k-1}v_j}\\
        \stackrel{(b)}\geq \sum_{i=1}^{L-k+1}\frac{v_i}{\sum_{j=i}^{i+k-1}v_j}+\sum_{i=L-k+2}^{L}\frac{v_i}{v_{i+k}+\sum_{\substack{j=i\\ j\neq 0}}^{i+k-1}v_j}\\
        \stackrel{(c)}= S_{V'}(L,k)\\
        \stackrel{(d)}> 1
    \end{align*}
    Here $(a)$ follows from $\frac{v_0}{v_0+\sum_{j=1}^{k-1}v_j}> 0$, $(b)$ follows from $v_0 = min_{i=0}^{L}{v_i}$, $(c)$ follows by assuming $V' = v_1,v_2,\cdots, v_L$ and $(d)$ follows from the induction assumption for the lower bound.  
\end{enumerate}
\end{itemize}
\end{IEEEproof}
\begin{lem}\label{lem:curl_d_general_k}
Given $\C,\A,k\geq 3$ and $\ell\geq k$, then for
\begin{itemize}
\item $\ell = k:\quad\quad\quad\curl_d(\C,\A,k) = 1.$
\item $\ell > k: \quad\quad1< \curl_d(\C,\A,k) < \ell-k+1.$
\end{itemize}
\end{lem}
\begin{IEEEproof}
The statement follows from Lemma \ref{lem:curl_d_general_k} and the definition of $\curl_d(\C,\A,k)$ given in Equation \ref{eq:curl_d_general_k}.
\end{IEEEproof}
