# Supplementary material for: Expert Graphs: Synthesizing New Expertise via Collaboration
Source: arXiv:2107.07054 source file (2021-07-15)
Supplement: Supplementary file 2 [file nontransitivity.tex]

{\color{black}
In the previous subsections, we show that the curl condition derived in Corollary \ref{cor:curl_bound_d_main} is both necessary and sufficient for any cycle $\A$. This gives us tight upper and lower bounds on an unknown edge on cycle $\A$ given other edges as given in Theorem \ref{thm:ub_main} below.
\begin{thm}\label{thm:ub_main}
Given $\ell$, $\mathcal{A}$, the expert provides $\hat{f}_d(C_{a_i},C_{a_{i+1}})$ for $i\in [\ell-1]$. Then, we have 
%$$\frac{l}{2}-\sum_{i=1}^{l-1}\hat{f}_d^{(a_i,a_{i+1})}\leq
\comment{\begin{align*}\max{(0,1-\sum_{i=0}^{l-2}\hat{p}_d^{(a_i,a_{i+1})})}\leq\hat{p}_d^{(a_{\ell-1},a_0)} \\\leq \min{(1,l-1-\sum_{i=1}^{\ell-1}\hat{p}_d^{(a_i,a_{i+1})})}.
\end{align*}}
\small{\[1-\sum_{i=0}^{\ell-2}\hat{f}_d(C_{a_i},C_{a_{i+1}})<\hat{f}_d(C_{a_{\ell-1}},C_{a_0})\\< \ell-1-\sum_{i=0}^{\ell-2}\hat{f}_d(C_{a_i},C_{a_{i+1}})\].}

\end{thm}
\begin{IEEEproof}
The proof follows from Corollary \ref{cor:curl_bound_d_main}.
\end{IEEEproof}}%{\color{red} Why is Theorem 5 here? Shouldn't this be in the section on the algorithm for filling in incomplete knowledge graphs? - Bijan}

The curl condition allows a degree of non-transitivity in pairwise experts. To explore this, we will first quantify non-transitivity in pairwise experts.

\begin{defn}
For an input distribution $d(\X)$, classes $\C$, and cycle of classes $\mathcal{A}$, we say the \textbf{strength of non-transitivity}, $\sigma_d^{(\C, \A)}$ is
\begin{equation}
    \sigma_d^{(\C, \A)} = \max\{{\min_{i \in [\ell]} \hat{f}_d(C_{a_i}, C_{a_{i+1}}), \min_{i \in [\ell]} \hat{f}_d(C_{a_{i+1}}, C_{a_i})}\}
\end{equation}
Note that $\sigma_d^{(\C, \A)} = \sigma_d^{(\C,\Ac)}$ by definition.
\end{defn}
\begin{defn}
We say that a cycle $\mathcal{A}$ is \textbf{non-transitive} if $\sigma_d^{(\C, \A)} > .5.$
\end{defn}

Intuitively, these definitions capture the notion of non-transitivity of preferences. If for classes $C_0$, $C_1$, $C_2$ we have $\sigma_d^{(\C, (0, 1, 2))} > .5$, this means that we have a ``cycle of preference." That is, we prefer ($\leftarrow$) $C_0 \leftarrow C_1\leftarrow C_2\leftarrow C_0.$ No matter which class we decide on, we have a pairwise expert that suggests it is the incorrect choice. This notion is related to the Condorcet Paradox~\cite{Condorcet}.
\begin{exmp}
Below we provide examples of \emph{non-transitive} cycles. 
\begin{itemize}
    \item $\fdv = (0.6,0.8,0.55)^T$: $\sigma_d^{(\C,\A)} = 0.55.$
     \item $\fdv = (0.3,0.4,0.4)^T$: $\sigma_d^{(\C,\A)} = 0.6.$
      \item $\fdv = (0.8,0.7,0.7,0.7)^T$: $\sigma_d^{(\C,\A)} = 0.7.$
\end{itemize}
\end{exmp}
%Note that in Example~\ref{exmp:nontransitive}, $\curl_{x}(\mathcal{C}, (1, 2, 3)) \rightarrow \frac{2}{3}$ for all $x \in \{x_1, x_2, x_3\}$. The curl captures the \emph{potential for non-transitivity} in that the label probabilities can be cycled through $x_1, x_2, x_3$ as in Example~\ref{exmp:nontransitive} so that $\hat{f}_d(x_i, x_{i+1}) = \curl_x(\mathcal{C}, (1, 2, 3))$. The following lemma will make this more precise.
\begin{obs}\label{obs:curllb}
For a cycle of length $\ell$, by definition we have $$\frac{\max\{\curl_d(\C,\A),\curl_d(\C,\Ac)\}}{\ell}\geq \sigma_d^{(\C,\A)}.$$
\end{obs}
\begin{cor}
Given $\ell \geq 3$, $\C$, $\A$, the strength of non-transitivity $\sigma_d^{(\C,\A)}$ is upper bounded by 
\[\sigma_d^{(\C,\A)} < \frac{\ell-1}{\ell}.\]
\end{cor}
\comment{\begin{IEEEproof}
The proof follows from Observation \ref{obs:curllb} and Corollary \ref{cor:curl_bound_d_main}. 
\end{IEEEproof}}

%From Observation~\ref{obs:curllb}, we see that non-transitivity is possible because of our ability to achieve $\curl_x(\C, \A)/\ell > .5$ with $f(C_i, C_j) = \hat{f}_x(C_i,C_j)$. The re-normalization that occurs in pairwise experts is responsible for this ``nontransitive'' curl. In addition, one also needs uncertainty in the input $x$ in order to average the curl into a stronger non-transitivity.
